# Supplementary material for: Nonlocal Josephson effect in Andreev molecules
Source: arXiv:1809.11011 ancillary file (2019-09-04)
Supplement: Supplementary file 1 [file suppinfo.pdf]

# Supporting Information
# Non-local Josephson effect in Andreev molecules

J.-D. Pillet,[†,‡] V. Benzoni,[†] J. Griesmar,[†] J.-L. Smirr,[†] and Ç. Ö. Girit*[,†]

†$\Phi_0$, *JEIP, USR 3573 CNRS, PSL Research University, 11, place Marcelin Berthelot, 75231 Paris Cedex 05, France*

‡*Laboratoire des Solides Irradiés, CNRS, CEA, Université Paris-Saclay, 91128 Palaiseau, France*

E-mail: caglar.girit@college-de-france.fr

## Contents

**1 Dependence of Andreev molecule spectra on separation 2**

**2 Discrete spectrum of Andreev molecules $|E| < \Delta$ 3**

2.1 Spectral asymmetry in junctions with perfect transmission . . . . . . . . . . 8

**3 Eigenstates and current carried by the continuum $|E| > \Delta$ 9**

**4 Andreev molecules in tunnel Josephson junctions 13**

4.1 Spectrum for small transmission $\tau_0 \ll 1$ . . . . . . . . . . . . . . . . . . . . . . . . 13

4.2 Off resonance ballistic devices . . . . . . . . . . . . . . . . . . . . . . . . 16

4.3 On resonance ballistic devices . . . . . . . . . . . . . . . . . . . . . . . . 18

4.4 Diffusive devices . . . . . . . . . . . . . . . . . . . . . . . . . . . . . . 19

# 1 Dependence of Andreev molecule spectra on separation

To show how the Andreev molecule spectra evolve as the separation is reduced and to better understand Figure 2 of the main text, Figure S1(a) to (e) plots the spectra for fixed $\delta_R = 3\pi/5, \tau_L = \tau_R \approx 0.94$ and five values of separation $l$. Subfigures for two values of the separation, (a) $l \gg \xi_0$ and (c) $l = \xi_0$, are already plotted in Figure 1 of the main text and three subfigures, (b) $l = 2\xi_0$ and (d) $l = 0.5\xi_0$ are new.

For moderate separation $l = 2\xi_0$ (b) ABS of the left and right junction start to hybridize into bonding and anti-bonding states producing avoided crossings around the points of degeneracy $\delta_R = \mp\delta_L$ corresponding to Elastic Cotunneling (dEC) and double Crossed Andreev Reflection (dCAR), respectively. In the spectrum (c) $l = \xi_0$ additional dashed lines show the energy levels for the case of perfect transmission ($\tau_R = \tau_L = 1$) where the crossing at $\delta_L = \delta_R$ (dCAR) is preserved. This is due to the fact that the dCAR mechanism requires backscattering which is absent for perfect transmission. In contrast the avoided crossings at $\delta_L = -\delta_R$ produced by dEC, a momentum conserving process, are still present. The inequivalence of the two processes of dEC and dCAR lead to the unusual asymmetry about $\delta_L = \pi$ in the spectra for fixed $\delta_R$.

As the junction separation is reduced, the size of the avoided crossings increases until some of the ABS are partially pushed out of the superconducting gap and into the continuum. In (d) the size of the avoided crossing at $\delta_L = -\delta_R$ (dEC) is maximal. Because the avoided crossing is maximal at this separation the innermost Andreev bound states are closest to zero energy at $\delta_L = -\delta_R$. This gives rise to the minimum in the lower solid line in Figure 2(a) of the main text.

When the distance $l$ becomes negligible compared to $\xi_0$, the two junctions fuse into a single junction with twice the scattering amplitude and one pair of ABS pushed entirely into

the continuum. Instead of having two junctions in series with transmissions $\tau_0 \approx 0.94$ at large separation $l \gg \xi_0$, there is now a single junction with a larger scattering amplitude $U_L + U_R$ (or equivalently a smaller transmission $\tau_0' \approx 0.8$) and an additional continuum state. The spectrum (e) is effectively that of a single junction of transmission $\tau_0' < \tau_0$ shifted by $\delta_R = 3\pi/5$ to account for the fact that the total phase drop is $\delta = \delta_L - \delta_R$. Because of the reduced effective transmission, the innermost Andreev bound states for phase $\delta_L = -\delta_R$ are farther away from zero energy than for separation $l = 0.5\xi_0$, spectrum (d). This explains why the solid line in Figure 2(a) of the main text moves up in energy after passing through a minimum near $l = 0.5\xi_0$.

## 2 Discrete spectrum of Andreev molecules $|E| < \Delta$

As explained in the main text, in order to find the discrete spectrum of Andreev molecules, we build wave functions from the eigenstates of an infinite superconductor, which are plane waves of electron or hole type ($\eta = e$ or $h$):

$$\psi^{\delta}_{\eta\pm}(x) = \frac{1}{\sqrt{L}} \left(u^{\delta}_{\eta}, v^{\delta}_{\eta}\right)^T e^{\pm i k_\eta x}$$

where $L$ is the total size of the system and we have defined coherence factors

$$u^{\delta}_{e(h)} = \frac{e^{-i\delta/2}}{\sqrt{2}} \left(1 \pm \sqrt{1-\epsilon^{-2}}\right)^{1/2}$$
$$v^{\delta}_{e(h)} = \mathrm{sign}(\epsilon) \times \frac{e^{i\delta/2}}{\sqrt{2}} \left(1 \mp \sqrt{1-\epsilon^{-2}}\right)^{1/2}$$

where $k_{e(h)}$ are complex momenta. If the superconducting gap is much smaller than the Fermi energy $\Delta \ll E_F$, they can be approximated as $k_{e(h)} \approx k_F \pm i/\xi$ where $k_F$ is the Fermi momentum in the normal state and the coherence length is a function of energy $\xi^{-1} = \xi_0^{-1}\sqrt{1-\epsilon^2} \ll k_F$. Here $\xi_0 = \hbar v_F/\Delta$ is the bare superconducting coherence length, $v_F$ is the Fermi velocity and $\epsilon = E/\Delta$ is the normalized energy. The wave-functions of Andreev

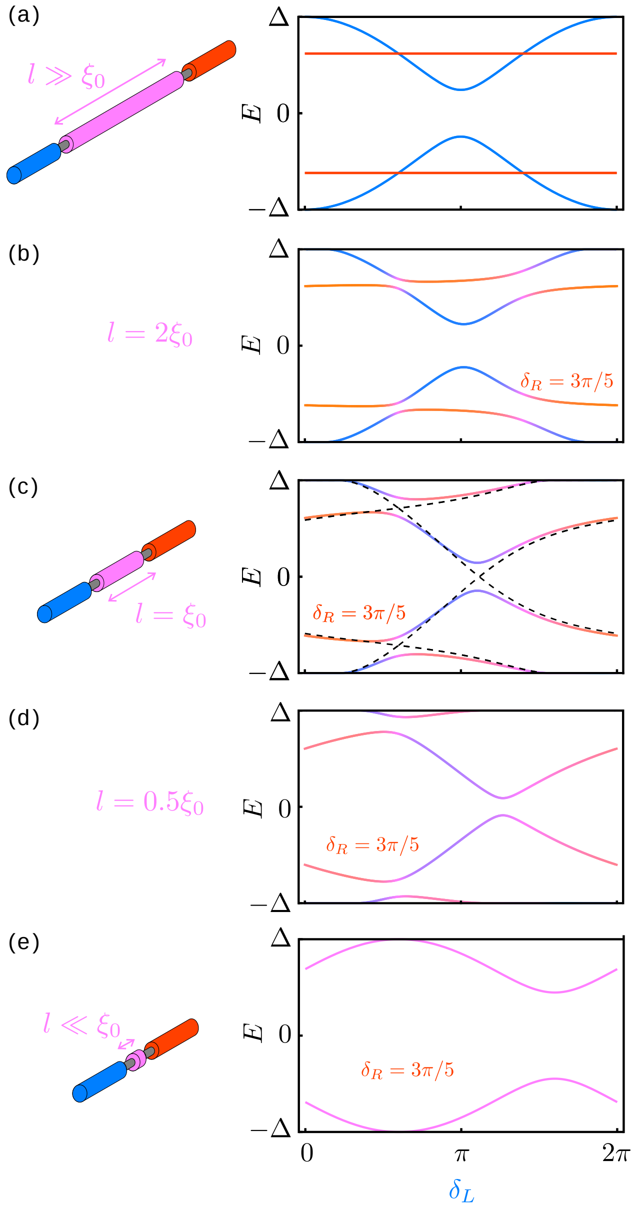


Figure S1: Energy spectrum of an Andreev molecule for varying separation. (a) When two single channel superconducting junctions are placed far from each other, their ABS are independent. Energies of ABS in the left junction (blue lines) modulate with $\delta_L$ (x-axis) while those of the right junction are constant (red lines). (b-c-d) When the junction separation $l$ is comparable to $\xi_0$, the ABS hybridize, leading to the appearance of avoided crossings at $\delta_L = \pm\delta_R$ which grow as $l$ decreases (magenta regions). Since the phases are $2\pi$ periodic, the $\delta_L = -\delta_R$ degeneracy is shown at $\delta_L = 2\pi - \delta_R = 7\pi/5$. The external ABS are gradually pushed into the continuum ($|E| > \Delta$) as a result of hybridization. The dashed line in graph (c) ($l = \xi_0$) shows the spectrum for perfect transmission ($\tau_L = \tau_R = 1$) where the $\delta_L = \delta_R$ splitting is absent. (e) For $l \ll \xi_0$, the two junctions merge into a single one, leaving only one pair of ABS. Parameters used for these calculations are $U_L = U_R = 0.25\hbar v_F$ ($\tau_L = \tau_R \approx 0.94$), $\delta_R = 3\pi/5$ and the Fermi momentum is chosen such that $k_F l \gg 1$ and $k_F l = \pi/2 \pmod{2\pi}$, maximizing the avoided crossings at $\delta_L = \delta_R$.

molecules are defined piecewise in the following way

$$\psi(x) = \begin{cases} l_e \psi_e^-(x) + l_h \psi_h^+(x) & \text{if } x < -l/2 \\ c_e^+ \psi_e^+(x) + c_e^- \psi_e^-(x) & \\ +c_h^+ \psi_h^+(x) + c_h^- \psi_h^-(x) & \text{if } |x| < l/2 \\ r_e \psi_e^+(x) + r_h \psi_h^-(x) & \text{if } l/2 < x \end{cases}$$

where we exclude diverging spinors on the left and the right and we introduce two sets of four coefficients $\Psi_e = (l_e, r_e, c_e^+, c_e^-)^T$ and $\Psi_h = \left(l_h, r_h, c_h^-, c_h^+\right)^T$ giving the respective weight of each component ($l$ for left, $r$ for right and $c^\pm$ for the center).

These wave-functions must be continuous at $x = \pm l/2$ in order to avoid unphysical sharp variation of the electronic density. This continuity can be expressed in the following way

$$\psi\left(\pm l/2^-\right) = \psi\left(\pm l/2^+\right)$$

where the superscripts $\pm$ mean slightly lower or larger than $\pm l/2$. Similarly, the Bogoliubov-de Gennes equation imposes boundary conditions on the derivative of $\psi$

$$\partial_x \psi\left(\pm l/2^+\right) - \partial_x \psi\left(\pm l/2^-\right) = \frac{2m}{\hbar} U_{R(L)} \psi(\pm l/2)$$

due to the $\delta$ Dirac function that we use to model scattering on the weak links. For the term on the right, we choose the definition

$$\psi(\pm l/2) = \left[\psi\left(\pm l/2^-\right) + \psi\left(\pm l/2^+\right)\right]/2$$

As said in the main text, these two conditions give eight equations for eight unknown coefficients

$$\Psi_e = a(\epsilon) A \Psi_h \quad \text{and} \quad \Psi_h = a(\epsilon) A^* \Psi_e \tag{1}$$

with $a(\epsilon) = e^{-i\arccos\epsilon}$ the probability amplitude for an electron to be Andreev reflected into a hole at the interface between a normal metal and superconductor. The matrix $A(\Phi) = e^{-i\Phi}M^{-1}M^{*}e^{i\Phi}$ depends on superconducting phase differences contained in the diagonal matrix $\Phi = \mathrm{diag}(\delta_L/2, \delta_R/2, 0, 0)$ and scattering amplitude at the weak links through matrix $M$

$$M = e^{ik_F l/2}\begin{pmatrix} i & 0 & -ie^{-ik_e l} & -i \\ 0 & i & -i & -ie^{-ik_e l} \\ -u_L & 0 & -u_L e^{-ik_e l} & u_L^{*} \\ 0 & u_R & -u_R^{*} & u_R e^{-ik_e l} \end{pmatrix}$$

with reduced scattering potentials

$$u_{L(R)} = 1 + iU_{L(R)}/\hbar v_F,$$

which are directly related to the transmissions of each junction $\tau_{L(R)} = 1/\left|u_{L(R)}\right|^2$. Combining the two parts of Eq. 1, we have non trivial solutions only if

$$\mathrm{Det}\left(1 - a(\epsilon)^2 A(\Phi) A^{-1}(-\Phi)\right) = 0. \quad (2)$$

This is equivalent to find energies for which

$$a(\epsilon)^2 \lambda_A = 1,$$

where $\lambda_A$ are eigenvalues of $A(\Phi) A^{-1}(-\Phi)$ and $\lambda_A \in U(1)$.

Writing equation $\mathrm{Det}(A(\Phi) - \lambda_A A(-\Phi)) = 0$, we can show that $\lambda_A$ are roots of a symmetric polynomial

$$\alpha_0\lambda_A^4 + \alpha_1\lambda_A^3 + \alpha_2\lambda_A^2 + \alpha_1\lambda_A + \alpha_0 = 0$$

with coefficients given by

$$\alpha_0 = \left| u_L u_R e^{-i2k_F l} - e^{-\frac{2l}{\xi}} \left(u_L - 1\right)\left(u_R - 1\right) \right|^2$$

and

$$\begin{cases} \alpha_1 = & -4\alpha_0 + \epsilon_1 \\ \epsilon_1 = & 4e^{-\frac{2l}{\xi}} \sin^2\left(\frac{\delta_R - \delta_L}{2}\right) \\ & -4\left[\left(1 - e^{-\frac{4l}{\xi}}\right)\left(u_L - 1\right)^2 + \left(e^{-\frac{2l}{\xi}} - 1\right)\right] \sin^2\left(\frac{\delta_R}{2}\right) \\ & -4\left[\left(1 - e^{-\frac{4l}{\xi}}\right)\left(u_R - 1\right)^2 + \left(e^{-\frac{2l}{\xi}} - 1\right)\right] \sin^2\left(\frac{\delta_L}{2}\right) \end{cases}$$

and

$$\begin{cases} \alpha_2 = & -2\left(\alpha_1 + \alpha_0 - \epsilon_2\right) \\ \epsilon_2 = & 8\left(e^{-\frac{2l}{\xi}} - 1\right)^2 \sin^2\left(\frac{\delta_R}{2}\right) \sin^2\left(\frac{\delta_L}{2}\right). \end{cases}$$

Since $\lambda_A \in U(1)$, the symmetric polynomial can be simplified to obtain the eigenenergies of the Andreev molecule,

$$\epsilon^2 = 1 - \frac{1}{8\alpha_0}\left(\epsilon_1 \pm \sqrt{\epsilon_1^2 - 8\alpha_0\epsilon_2}\right). \tag{3}$$

In the general case, solutions to this transcendental equation can only be found numerically. It is however useful to obtain analytical results in particular cases such as infinitely close ($l \approx 0$) or far junctions ($l \to \infty$), and we will see in one of the following appendices that we can use it to obtain analytical formula for the Andreev molecule spectrum of two closely spaced tunnel junctions.

From the solutions of Eq. 2, we generally obtain up to four eigenenergies $E_{ABS}$, from which we can deduce the contribution of ABS to the supercurrent flowing through the left

junction,

$$I_L^{ABS} = -\frac{1}{\varphi_0} \sum_{E_{ABS}<0} \frac{\partial E_{ABS}}{\partial \delta_L}.$$

In an Andreev molecule, the energies $E_{ABS}$ depend both on $\delta_L$ and $\delta_R$, which leads to non-local phase dependencies of the supercurrent.

## 2.1 Spectral asymmetry in junctions with perfect transmission

In the general case, Eq. 2 does not have simple analytical solutions and it requires a numerical resolution to find Andreev molecule spectra. However, in the limit of large transmission $\tau_0 \to 1$ (or equivalently $u_{L(R)} = 1$), it simplifies into two compact transcendental equations

$$e^{-2\frac{l}{\xi_0}\sin\beta} \sin\frac{\delta_L}{2} \sin\frac{\delta_R}{2} = \sin\left(\frac{\delta_L}{2} \mp \beta\right) \sin\left(\frac{\delta_R}{2} \pm \beta\right) \tag{4}$$

where $\beta = -\arccos\epsilon$ and $\epsilon = E/\Delta$, from which one can deduce interesting spectral features. For example, we can recover spectra for well known particular cases. If the junctions are infinitely far ($l \to \infty$), the left-hand side cancels and we get $\epsilon = \pm\cos\frac{\delta_{L(R)}}{2}$, which are the usual ABS for two independent perfectly transmitted junctions. Similarly, if the junctions are merged into a single one ($l = 0$), we recover the spectrum $\epsilon = \pm\cos\left(\frac{\delta_L - \delta_R}{2}\right)$ of a single junction with a phase drop $\delta_L - \delta_R$.

Eq. 4 can also yield interesting prediction about Andreev molecules in the general case such as the spectral asymmetry that we mention in the main part of this manuscript. As shown in Fig. 1(c) (main text) the Andreev bound state spectrum for independent junctions is symmetric about $\delta = \pi$ and $\epsilon = 0$. The ABS cross at this point for perfect transmission ($\tau_0 = 1$). For two closely spaced junctions however, this symmetry is broken and the degeneracy point is shifted along the phase axis. If the phase $\delta_R$ across the right junction is fixed, ABS become degenerate at $\epsilon = 0$ (*i.e.* $\beta = -\pi/2$) and

$$\delta_L = \pi - 2\arctan\left[e^{-2l/\xi_0}\tan\frac{\delta_R}{2}\right]$$

Due to ABS hybridization, the degeneracy point shifts from $\pi$ of $\varphi \approx 2\arctan\left[e^{-2l/\xi_0}\tan\frac{\delta_R}{2}\right]$, which makes the spectrum asymmetric. We notice that this deviation is significant only if two junctions are sufficiently close ($l \approx \xi_0$) but decreases exponentially when $l$ becomes large compared to $\xi_0$.

# 3 Eigenstates and current carried by the continuum $|E| > \Delta$

The continuum of Andreev molecules is obtained with a similar approach as for the sub-gap states but with energies larger than the superconducting gap $|E| > \Delta$. We look for wavefunctions $\psi_E$ that are continuous along the $x$-axis and obey the Bogoliubov-De Gennes (BDG) equation $H\psi_E = E\psi_E$, where $E$ is the eigenenergy and $H$ is given by Eq. 1 (main text). They are built from the eigenstates of an infinite superconductor, which are plane waves of electron or hole type ($\eta = e$ or $h$)

$$\psi^{\delta}_{\eta\pm}(x) = \frac{1}{\sqrt{L}}\left(u^{\delta}_{\eta}, v^{\delta}_{\eta}\right)^{T} e^{\pm ik_{\eta}x}$$

where $L$ is the total size of the system and we have defined coherence factors

$$u^{\delta}_{e(h)} = \frac{e^{-i\delta/2}}{\sqrt{2}}\left(1 \pm \sqrt{1-\epsilon^{-2}}\right)^{1/2}$$
$$v^{\delta}_{e(h)} = sign(\epsilon) \times \frac{e^{i\delta/2}}{\sqrt{2}}\left(1 \mp \sqrt{1-\epsilon^{-2}}\right)^{1/2}$$

Assuming $\Delta \ll E_F$, we can make the approximation $k_{e(h)} \approx k_F \pm 1/\xi$ where $k_F$ is the Fermi momentum in the normal state and the coherence length is a function of energy $\xi^{-1} = \xi_0^{-1}\sqrt{1-\epsilon^2} \ll k_F$. Here $\xi_0 = \hbar v_F/\Delta$ is the bare superconducting coherence length, $v_F$ is the Fermi velocity and $\epsilon = E/\Delta$ is the normalized energy.

Since momenta $k_\eta$ are real, there is no bound states but only propagating solutions called scattering states. They are superpositions of an incoming wave and an outgoing wave

resulting from scattering at the weak links

$$\psi_E^{\eta\pm} = \psi_{inc}^{\eta\pm}(x) + \psi_{out}^{\eta\pm}(x) \tag{5}$$

with four possible types of incoming wave (here $\Theta$ is the Heaviside step function)

$$\begin{aligned}
\psi_{inc}^{e+}(x) &= \psi_{e+}^{\delta_L}(x)\,\Theta\left[-x - l/2\right] \\
\psi_{inc}^{e-}(x) &= \psi_{e-}^{\delta_R}(x)\,\Theta\left[x - l/2\right] \\
\psi_{inc}^{h+}(x) &= \psi_{h+}^{\delta_R}(x)\,\Theta\left[x - l/2\right] \\
\psi_{inc}^{h-}(x) &= \psi_{h-}^{\delta_L}(x)\,\Theta\left[-x - l/2\right]
\end{aligned}$$

and resulting outgoing wave

$$\psi_{out}^{\eta\pm}(x) = \begin{cases} c_1^{\eta\pm}\psi_{e-}^{\delta_L}(x) + c_2^{\eta\pm}\psi_{h+}^{\delta_L}(x) & \text{for } x < -\frac{l}{2} \\ c_3^{\eta\pm}\psi_{e-}^{0}(x) + c_4^{\eta\pm}\psi_{h+}^{0}(x) & \\ +c_5^{\eta\pm}\psi_{e+}^{0}(x) + c_6^{\eta\pm}\psi_{h-}^{0}(x) & \text{for } |x| < \frac{l}{2} \\ c_7^{\eta\pm}\psi_{e+}^{\delta_R}(x) + c_8^{\eta\pm}\psi_{h-}^{\delta_R}(x) & \text{for } x > \frac{l}{2} \end{cases}$$

For each type of incoming wave, we have a set of eight coefficients

$$\Psi_E^{\eta\pm} = \left(c_1^{\eta\pm}, c_2^{\eta\pm}, c_3^{\eta\pm}, c_4^{\eta\pm}, c_5^{\eta\pm}, c_6^{\eta\pm}, c_7^{\eta\pm}, c_8^{\eta\pm}\right)^T$$

giving the respective weight on the left, right and in the center of the device for the outgoing wave. The continuity of the wavefunctions and the conditions imposed on their derivatives by the BDG equation[1] give the relations

$$\Psi_E^{\eta\pm} = -M_E^{-1}\Psi_{inc}^{\eta\pm} \tag{6}$$

where $M_E$ is a $8 \times 8$ matrix given by ($0_2$ are $2 \times 2$ matrix of zeros)

$$M_E = \begin{pmatrix} m_{\delta_L} m_k^+ & -m_k^+ & -m_k^- & 0_2 \\ 0_2 & -m_k^- & -m_k^+ & m_{\delta_R} m_k^+ \\ m_{\delta_L} m_k^+ m_u^L & -m_k^+ m_u^{L*} & m_k^- m_u^L & 0_2 \\ 0_2 & m_k^- m_u^R & -m_k^+ m_u^{R*} & m_{\delta_R} m_k^+ m_u^R \end{pmatrix}$$

and we define three submatrices depending on the parameters of the device

$$m_u^{L(R)} = \begin{pmatrix} u_{L(R)} & 0 \\ 0 & -u_{L(R)}^* \end{pmatrix} \quad m_\delta = \begin{pmatrix} e^{\frac{i\delta}{2}} & 0 \\ 0 & e^{-\frac{i\delta}{2}} \end{pmatrix}$$

$$m_k^\pm = \begin{pmatrix} e^{\pm\frac{ik_e l}{2}} & a\left(\epsilon\right) e^{\mp\frac{ik_h l}{2}} \\ a\left(\epsilon\right) e^{\pm\frac{ik_e l}{2}} & e^{\mp\frac{ik_h l}{2}} \end{pmatrix}$$

The vectors $\Psi_{inc}^{\eta\pm}$ can have four different forms depending on the nature of the incoming waves ($e$ or $h$) and their directions of propagation ($+$ for $x > 0$ and $-$ for $x < 0$)

$$\Psi_{inc}^{e+} = e^{-i\frac{k_e l + \delta_L}{2}} \begin{pmatrix} e^{i\delta_L} \\ a_\epsilon \\ 0 \\ 0 \\ -u_L^* e^{i\delta_L} \\ -u_L^* a_\epsilon \\ 0 \\ 0 \end{pmatrix}$$

$$\Psi_{inc}^{e-} = e^{-i\frac{k_e l+\delta_R}{2}} \begin{pmatrix} 0 \\ 0 \\ e^{i\delta_R} \\ a_\epsilon \\ 0 \\ 0 \\ -u_R^* e^{i\delta_R} \\ -u_R^* a_\epsilon \end{pmatrix}$$

$$\Psi_{inc}^{h-} = e^{i\frac{k_h l-\delta_L}{2}} \begin{pmatrix} a_\epsilon e^{i\delta_L} \\ 1 \\ 0 \\ 0 \\ u_L a_\epsilon e^{i\delta_L} \\ u_L \\ 0 \\ 0 \end{pmatrix}$$

$$\Psi_{inc}^{h+} = e^{i\frac{k_h l-\delta_R}{2}} \begin{pmatrix} 0 \\ 0 \\ a_\epsilon e^{i\delta_R} \\ 1 \\ 0 \\ 0 \\ u_R a_\epsilon e^{i\delta_R} \\ u_R \end{pmatrix}$$

with $a_\epsilon = \mathrm{sign}\,(\epsilon) \left|\epsilon - \sqrt{\epsilon^2 - 1}\right|$ the probability amplitude for an electron of normalized energy $\epsilon$ to be Andreev reflected at the interface between a normal metal and a superconductor.

This gives then four degenerate states for each energy $E$.

The solutions obtained from Eq. 5 with sets of coefficients 6 can therefore be written in the following way

$$\psi_E^{\eta\pm}(x) = \frac{1}{\sqrt{L}} \begin{pmatrix} U_E^{\eta\pm}(x) \\ V_E^{\eta\pm}(x) \end{pmatrix},$$

where $U_E^{\eta\pm}$ is the electron part and $V_E^{\eta\pm}$ is the hole part of the wavefunctions. In one dimension and at zero temperature, the current at equilibrium carried by these states is given by[2,3]

$$I(x) = \tfrac{2e\hbar}{mL} \textstyle\sum_{\eta,\sigma} \sum_{|k|>k_F} \mathrm{Im}\left[V_E^{\eta\sigma}(x)^* \partial_x V_E^{\eta\sigma}(x)\right] \cdot$$

The current flowing through the left junction is obtained by evaluating this expression at $x = -l/2$. We substitute the sum by an integral $\sum_k \to \int_k dk \times L/2\pi$ and sum over energy rather than momentum by making use of $d\xi_k/dk \approx \hbar^2 k_F/m$ and $d\xi_k/dE = E/\sqrt{E^2-\Delta^2}$ where $\xi_k$ is the kinetic energy. The current carried by the continuum through the left junction is therefore given by

$$I_L^{cont} = \tfrac{1}{\varphi_0} \textstyle\sum_{\eta\sigma} \int_\Delta^\infty \tfrac{dE}{2\pi k_F} \tfrac{E}{\sqrt{E^2-\Delta^2}} \\ \mathrm{Im}\left[V_E^{\eta\sigma}\left(-\tfrac{l}{2}\right)^* \partial_x V_E^{\eta\sigma}\left(-\tfrac{l}{2}\right)\right]$$

where $\varphi_0 = \hbar/2e$ is the flux quantum. The current through the right junction $I_R$ is obtained similarly by taking $x = +l/2$.

# 4 Andreev molecules in tunnel Josephson junctions

## 4.1 Spectrum for small transmission $\tau_0 \ll 1$

A wide variety of superconducting devices including most superconducting qubits are based on tunnel Josephson junctions. In that case, ABS are very close to the edge of the superconducting gap ($\epsilon \sim 1$) such that their wave-functions extend over a large distance ($\xi_0/\xi \ll 1$).

For devices made, for example, with aluminum, the distance $l$ between the junction is typically comparable to the bare superconducting coherence length $\xi_0$ and the overlap of ABS wave-functions $e^{-2l/\xi} \sim 1$ becomes important (Figure S2(a)). One could thus naively expect a strong hybridization of their ABS leading to spectacular non-local effects. However, for small transmission $\tau_0$, non-local microscopic mechanisms (dEC and dCAR) are very unlikely as they require double tunneling of Cooper pairs through the barriers with a probability proportional to $\tau_0^2$. This competes with local tunneling of Cooper pairs (EC) whose probability is proportional to $\tau_0 \left(1 - e^{-2l/\xi}\right)$ where the second factor corresponds to the portion of the ABS wave-functions in the central superconductor. As a consequence, local events will generally dominate unless wave-functions spread over a very large distance $\xi \sim l/\tau_0$. In standard devices, the distance between tunnel junctions is a few $\mu$m and the transmissions are around $\tau_0 \sim 10^{-6}$ (for 1 $\mu$A.$\mu$m$^{-1}$). Wave-functions would thus have thus to extent over more than a meter in order to fulfill this condition, which suggests that non-local effects are weak in these devices and one expects to observe standard Josephson effect.

This reasoning does not take into account the fact that the tunnel barriers form a Fabry-Perot cavity, which leads to interference that drastically affects the transmission. This interference results in the formation of normal discrete electronic levels in the central part of the device that will serve as channels for local and non-local microscopic events to happen. As we will see in this appendix, one can distinguish "off" or "on" resonance conditions, depending on the value of $k_F l$, for which the transmission is respectively reduced or increased and the Josephson effect, including non-local processes, is modified.

One advantage of the tunnel limit is that it provides compact analytical expression of the Andreev spectrum giving insight in the mechanism leading to ABS hybridization. In the tunnel limit $(l/\xi \ll 1)$ in Eq. 3 leads to the following ABS spectrum

$$\epsilon^{\pm\pm} \approx \pm\sqrt{1 - \tau\left(\epsilon^{\pm\pm}\right) \mathcal{F}_{\pm}\left(\delta_{L,}\delta_R\right)} \tag{7}$$

where energy has been normalized by the superconducting gap $\Delta$. This expression is an approximation, which remains correct if $\sin^2(k_F l) \neq 0$ or if the junctions are not too close $l/\xi \gg \tau_0$. Here, $\tau(\epsilon)$ is an energy-dependent effective transmission and $\mathcal{F}_\pm$ are combinations of trigonometric functions of $\delta_{L(R)}$

$$\mathcal{F}_\pm(\delta_L,\delta_R) = \mathcal{F}_1 \mp \sqrt{\mathcal{F}_1^2 - \mathcal{F}_2}$$

with

$$\begin{cases} \mathcal{F}_1 & = s_L^2 + s_R^2 + \frac{\tau_0 \xi}{4l} s_{LR}^2 \\ \mathcal{F}_2 & = 4\sin^2(k_F l)\, s_L^2 s_R^2 \end{cases}$$

where we have introduced compact notations

$$\begin{cases} s_L & = \sin\left(\frac{\delta_L}{2}\right) \\ s_R & = \sin\left(\frac{\delta_R}{2}\right) \\ s_{LR} & = \sin\left(\frac{\delta_L - \delta_R}{2}\right) \end{cases}$$

Intuitively, one can see that combinations of $s_{L(R)}$ and $s_{LR}$ will result in contributions proportional to $\sin(\delta_L \mp \delta_R)$, emerge respectively from dEC and dCAR and others to $\sin^2 \delta_{L(R)}$ linked to local processes. The secular Eq. 7 is similar to the energy spectrum of ABS in a single junction except that the apparent transmission $\tau(\epsilon)$ depends on $\xi$, and therefore on the energy, and momentum $k_F$. At first order in $l/\xi$, this transmission is given by

$$\tau(\epsilon) \approx \frac{\tau_0}{2} \frac{l/\xi}{(l/\xi)^2 + \sin^2(k_F l)} \tag{8}$$

This function of $k_F l$ peaks and becomes larger than the bare transmission of the junctions $\tau_0$ when $k_F l = 0 \ (\mathrm{mod}\pi)$ but still with $\tau(\epsilon) < 1$ thanks to the condition $l/\xi \gg \tau_0$. This results in periodic Lorentzian shaped peaks of width $l/\xi$. This width is reminiscent of the decay $e^{-l/\xi}$ of quasiparticles propagating between the tunnel barriers in the central part

of the device such that interference gradually disappears as $l$ tends to infinity. For other values of $k_F l$, $\tau(\epsilon)$ becomes much smaller. These variations of the transmission cause ABS to respectively go deeper into the superconducting gap or closer to its edge, which makes $\xi$ vary by orders of magnitude. At the same time, the probabilities for local and non-local processes to happen are also affected as they depend on how ABS wave-functions spread over the different parts of the device. This incidentally changes the nature of the Josephson effect as we will subsequently demonstrate.

## 4.2 Off resonance ballistic devices

Interference as described above would only be observable if quasiparticles could propagate ballistically in the device and preserve their phases. In hypothetical devices made with ballistic superconductors, effects of ABS hybridization through dEC and dCAR can have spectacular consequences on the properties of the circuits whether it is resonant or not.

Off resonance ($\sin^2(k_F l) \approx 1$, Figure S2(b)), the transmission can be approximated as $\tau \approx \tau_{off}\sqrt{1-\epsilon^2}$ with $\tau_{off} = \tau_0 l/(2\xi_0)$ and becomes much smaller than the bare transmissions of the junctions since $\epsilon \approx 1$. Under this condition, Eq. 7 at first order in $l/\xi$ leads to the following ABS energies

$$\epsilon_{off}^{\pm\pm} = \pm\sqrt{1-\tau_{off}^2\left[s_L^2+s_R^2 \mp \sqrt{\left(s_L^2-s_R^2\right)^2+\frac{\xi_0^2}{l^2}s_{LR}^2}\right]^2}$$

This is very different from the standard ABS spectrum of a single junction. First, energies depend on two superconducting phase differences $\delta_{L(R)}$ rather than a single one. Moreover the amplitude of ABS oscillation with these phases has an amplitude proportional to $\tau_0^2$ rather than $\tau_0$, which drastically suppresses the supercurrent carried by ABS. This is due to destructive interference in the Fabry-Perot resonator formed by the two barriers, and this suppression becomes more efficient as the junctions are placed closer to each other.

On top of these interference effects, the formation of an Andreev molecule, due to hy-

bridization of ABS, materializes in the term proportional to $s_{LR}$, due to dEC, with an amplitude that slowly tends to zero when junctions are far from each other compared to $\xi_0$. As shown in Figure S2, it manifests in the spectrum as avoided crossings between ABS of the left and right junctions at $\delta_L = -\delta_R$. Remarkably, the avoided crossing is much less pronounced at $\delta_L = \delta_R$ and even cancels at first order in $l/\xi$ (Figure S2(c)). This is because dCAR is strongly suppressed by destructive interference in the central part of the device, while dEC involving a direct tunneling between the left and right part remains important. Similarly to the case of junctions with large transmissions described before, for a fixed $\delta_R$, this introduces large asymmetry with respect to $\delta_L = \pi$ in the spectra. Note that here we can recover the spectrum of a single junction by taking $l \to 0$.

The contribution of ABS to the Josephson energy is given by the sum of ABS of negative energies $E_{ABS} = \Delta\left(\epsilon_{\mathit{off}}^{-+} + \epsilon_{\mathit{off}}^{--}\right)$ and, since $\tau_{\mathit{off}} \ll 1$, it can be approximated as

$$E_{ABS} \approx \frac{\Delta}{2}\tau_{\mathit{off}}^2 \left[\sum_{i=L,R}(1-\cos\delta_i)^2 + 2\frac{\xi_0^2}{l^2}s_{LR}^2\right]$$

where we have discarded a constant term. This expression has the same $2\pi$-periodicity with $\delta_{L(R)}$ than the Josephson energy of a single junction ($E_J \propto \cos\delta$) but also additional harmonics with a $\pi$-periodicity. As a consequence, the current carried by ABS deviates from the usual Josephson relation ($I_J = I_c \sin\delta$)

$$I_{L(R)}^{ABS} = I_c^{\mathit{off}}\left[4s_{L(R)}^2 \times \sin\delta_{L(R)} \pm \frac{\xi_0^2}{l^2}\sin\left(\delta_L - \delta_R\right)\right] \tag{9}$$

The off resonance critical current $I_c^{\mathit{off}} = \Delta\tau_{\mathit{off}}^2/2\varphi_0$ is much smaller than the bare critical current of individual Josephson junctions $I_c = \Delta\tau_0/4\varphi_0$ since $\tau_{\mathit{off}}^2 \ll \tau_0$ and would be therefore only detectable for moderately low transmissions, for example $\tau_0 \approx 0.1$. The second term in Eq. 9 is of non-local nature and is the consequence of ABS hybridization between the junctions. We see that if one junction is polarized with a finite phase, for example with $\delta_R \neq 0$, the ABS will carry a supercurrent through the other junction even when no phase is

applied across it (Figure S2(d)). Maintaining $\delta_L = 0$, ABS have thus a perfectly non-local behavior with a 0-phase current $I_L^{ABS}(0, \delta_R) = -I_c^{off} \xi_0^2 / (4l^2) \times \sin(\delta_R)$. This behavior is however extremely hard to detect experimentally because the continuum is carrying a much larger supercurrent than the ABS. Numerical calculations show us that the total current–phase relation is the same as the one of a single bare junction up to a factor (Figure S2(e)). In order to see the formation of Andreev molecules, we would need to be able to measure selectively the current carried by ABS and the continuum.

### 4.3 On resonance ballistic devices

The behavior of the device is completely different in the resonant case (Figure S2(f)). If $\sin^2(k_F l) \approx 0$, the transmission then peaks at $\tau \approx \tau_{on} \sqrt{1 - \epsilon^2}^{-1}$ with $\tau_{on} = \tau_0 \xi_0 / (2l)$. In this configuration, two ABS merge with the continuum at $\epsilon = 1$ leaving a spectrum of a single ABS pair

$$\epsilon_{on}^{\pm} = \pm \sqrt{1 - \left[2\tau_{on}\left(s_L^2 + s_R^2\right)\right]^{2/3}}$$

The exponent 2/3 of the second term under the square root is due to the joined effects of dEC and dCAR, which are enhanced by the fact that a resonant level lie at the Fermi energy level of the electrodes. This can be understood by looking at the evolution of the ABS spectrum under resonant condition when the left and right junctions are gradually brought together from infinity, which makes non-local processes more and more effective. This causes the formation of larger and larger avoided crossings between ABS of the left and right junction. Once the limit $l/\xi \ll 1$ has been reached, one pair of ABS vanishes into the continuum while the other one lies within the superconducting gap and always remains detached from the edge provided that one of the phases $\delta_{L(R)}$ is finite (Figure S2(g)). The remaining pair is fully delocalized over the two junctions. Moreover, due to constructive interference, the amplitude of ABS oscillations is proportional to $\tau_0^{2/3}$, which can be orders of magnitude larger than for isolated tunnel junctions. Note that, in this expression, we cannot take the

limit $l \to 0$ to merge the two junctions and recover the spectrum of a single one because the conditions of validity ($\sin^2(k_F l) \neq 0$ or $l/\xi \gg \tau_0$) would not be respected and we would obtain transmission $\tau(\epsilon) \sim \tau_0 \xi / l$ larger than 1, which is unphysical.

Similarly to the off resonance case, one can deduce the contribution of ABS to the Josephson energy

$$E_{ABS} \approx -\frac{\Delta}{2}\tau_{on}^{2/3}\left(2 - \cos\delta_L + \cos\delta_R\right)^{2/3}$$

as well as the current carried by ABS

$$I_{L(R)}^{ABS} = I_c^{on} \sin\delta_{L(R)}\left(2 - \cos\delta_L - \cos\delta_R\right)^{-1/3} \tag{10}$$

with the critical current $I_c^{on} = \Delta\tau_{on}^{2/3} / (3\varphi_0)$. Similarly to the off resonance case, the contribution of the continuum is important and the total current–phase relation is the same as the one of a single bare junction (Figure S2(e) and (h)).

In practice, ballistic superconductors are extremely rare in superconducting circuits, but semiconducting nanowires covered with epitaxial aluminum or Van der Waals materials such as $NbSe_2$ are potential candidates for the observation of an Andreev molecule in ballistic tunnel devices. Non-local effects are however much weaker than in devices of larger transmission and it would be a challenge to detect them. For example, the $\varphi-$junction behavior seems almost suppressed (Figure S2(e)).

## 4.4 Diffusive devices

In most experiments involving tunnel Josephson junctions, superconductors are diffusive. Each electronic channel carry a supercurrent through diffusive paths over which electrons take random phases $k_F l$ where $l$ can vary by several Fermi wavelengths. As a consequence, the interference effects that we described previously are suppressed and non-local effects are essentially negligible. The total Josephson energy of the system is obtained by averaging the

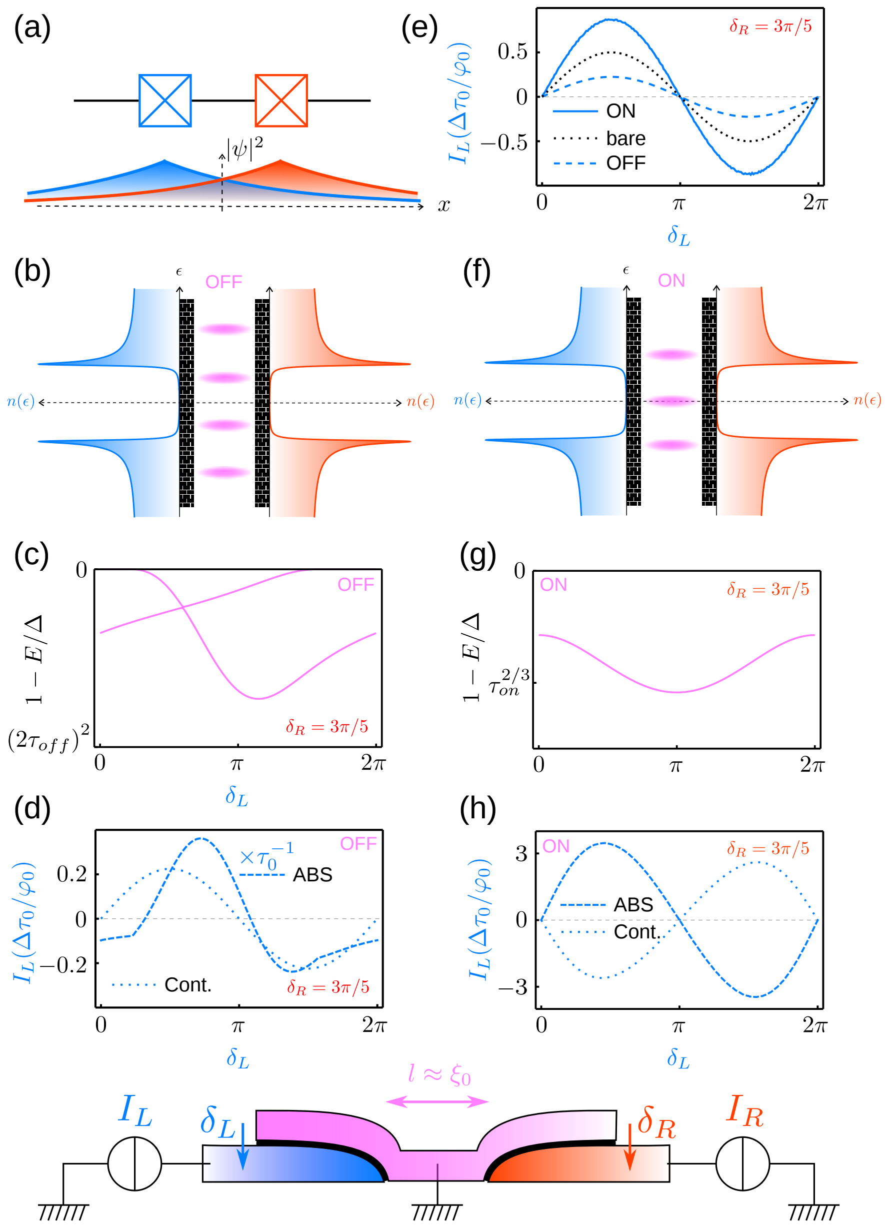


Figure S2: Andreev molecules in tunnel junctions. (a) For tunnel junctions, $\xi \gg \xi_0$, which can lead to a strong overlap of the ABS wavefunctions $\psi$ even for $l > \xi_0$. (b) When $\sin^2(k_F l) \approx 1$, the device is off resonance, the effective transmission is small and the Josephson effect is drastically reduced, as shown in the spectrum (c) and supercurrent-phase relation (d). (e) Comparing the supercurrent-phase relations ON (solid line) and OFF (dashed line) resonance, both are sinusoidal with with no $\varphi$-junction behavior. The critical current is larger on resonance and smaller off resonance as compared to a single tunnel junction with $\tau_0 \approx 10^{-4}$ (bare, dotted line). (f) On resonance, $\sin^2(k_F l) = 0$, the effective transmission is large and the spectrum (g) spectrum shows one pair of ABS which are detached from the edge of the gap. Both ABS and the continuum contribute to the supercurrent (h) but in opposite direction. Parameters used for these calculations: $\delta_R = 3\pi/5$, $l/\xi_0 = 1$, $U_L = U_R = 100\,\hbar v_F$ ($\tau_L = \tau_R \approx 10^{-4}$), and $k_F l \gg 1$.

phase over all channels

$$E_J \approx \frac{\Delta}{\pi} \int_{-\pi/2}^{\pi/2} (\epsilon^{-+} + \epsilon^{--}) dk_F l$$

where $\epsilon^{-\pm}$ are the energies of ABS of negative energies in Eq. 7 and the integral is summing over all the possible values of $k_F l$ within one period of $\tau(\epsilon)$. This can either be done numerically or by approximating $\tau(\epsilon)$ as a Dirac delta distribution $\tau_0 \pi \delta(k_F l)/2$ leading at first order in $\tau_0$ to

$$E_J \approx \frac{\tau_0 \Delta}{2} (\cos\delta_L + \cos\delta_R)$$

where we have dismissed a constant term. This simply corresponds to the Josephson energy of two independent tunnel Josephson junctions. The next-order correction in $\tau_0$ is given by

$$\delta E_J \approx \frac{\tau_0^{5/3} \xi_0^{2/3}}{8 l^{2/3}} \frac{s_{LR}^2}{\left(s_L^2 + s_R^2\right)^{1/3}}$$

which is completely negligible since $\tau_0^{5/3} \ll \tau_0$.

In fact, even taking into account the contribution of the continuum, the current-phases relations correspond to the standard Josephson formula $I_{L(R)} \approx I_c \sin\delta_{L(R)}$ where $I_c$ is the bare critical current of the junctions. The effects of ABS hybridization are therefore hardly measurable in conventional devices with superconducting tunnel junctions. It would be interesting however to explore the implications of a fraction of the supercurrent being carried by the continuum for SQUID measurements or the coherence time of superconducting qubits.

## References


(1) Blonder, G. E.; Tinkham, M.; Klapwijk, T. M. Transition from metallic to tunneling regimes in superconducting microconstrictions: Excess current, charge imbalance, and supercurrent conversion. *Phys. Rev. B* **1982**, *25*, 4515–4532.

(2) Bardeen, J.; Kümmel, R.; Jacobs, A. E.; Tewordt, L. Structure of Vortex Lines in Pure

Superconductors. *Physical Review* **1969**, *187*, 556–569.

(3) Beenakker, C. W. J.; van Houten, H. Josephson current through a superconducting quantum point contact shorter than the coherence length. *Phys. Rev. Lett.* **1991**, *66*, 3056–3059.
